# Supplementary material for: Search-Based Software Re-Modularization: A Case Study at Adyen
Source: arXiv:2102.00701 source file (2021-04-09)
Supplement: Supplementary file 1 [file appendix-fig-part1-all-pics.tex]

\begin{figure}[H]
     \centering
     \begin{subfigure}[b]{0.49\textwidth}
         \centering
         \includegraphics[width=\textwidth]{img/3dgraphs/run1-1.png}
     \end{subfigure}
     \hfill
     \begin{subfigure}[b]{0.49\textwidth}
         \centering
         \includegraphics[width=\textwidth]{img/3dgraphs/run1-2.png}
     \end{subfigure}
        \caption{Pareto front of the first run\protect\footnotemark}
        \label{fig:run1}
\end{figure}
\footnotetext{An interactive 3d visualization of these figures can be seen in the links in the footnotes of each figure. \url{https://github.com/SERG-Delft/ga-remodularization-appendix/blob/master/run1_3dview.html} \\ These figures can also be downloaded as a zip file from \url{https://doi.org/10.5281/zenodo.4011987
}}
\begin{figure}[H]
     \centering
     \begin{subfigure}[b]{0.49\textwidth}
         \centering
         \includegraphics[width=\textwidth]{img/3dgraphs/run1-3.png}
     \end{subfigure}
     \hfill
     \begin{subfigure}[b]{0.49\textwidth}
         \centering
         \includegraphics[width=\textwidth]{img/3dgraphs/run1-4.png}
     \end{subfigure}
        \caption{Solutions that improve on all metrics from the pareto front of the first run\protect\footnotemark}
        \label{fig:run1sub}
\end{figure}
\footnotetext{\url{https://github.com/SERG-Delft/ga-remodularization-appendix/blob/master/run1_3dview_filtered.html}}
\begin{figure}[H]
     \centering
     \begin{subfigure}[b]{0.49\textwidth}
         \centering
         \includegraphics[width=\textwidth]{img/3dgraphs/run2-1.png}
     \end{subfigure}
     \hfill
     \begin{subfigure}[b]{0.49\textwidth}
         \centering
         \includegraphics[width=\textwidth]{img/3dgraphs/run2-2.png}
     \end{subfigure}
        \caption{Pareto front of the second run\protect\footnotemark}
        \label{fig:run2}
\end{figure}
\footnotetext{\url{https://github.com/SERG-Delft/ga-remodularization-appendix/blob/master/run2_3dview.html}}
\begin{figure}[H]
     \centering
     \begin{subfigure}[b]{0.49\textwidth}
         \centering
         \includegraphics[width=\textwidth]{img/3dgraphs/run2-3.png}
     \end{subfigure}
     \hfill
     \begin{subfigure}[b]{0.49\textwidth}
         \centering
         \includegraphics[width=\textwidth]{img/3dgraphs/run2-4.png}
     \end{subfigure}
        \caption{Solutions that improve on all metrics from the pareto front of the second run\protect\footnotemark}
        \label{fig:run2sub}
\end{figure}
\footnotetext{\url{https://github.com/SERG-Delft/ga-remodularization-appendix/blob/master/run2_3dview_filtered.html}}

\begin{table}[H]
\caption{Relative improvement of best solutions for each optimization variable, that improve on all optimization variables.}
\label{bestgoodresults}
\begin{tabular}{@{}lrrr@{}}
\toprule
                            & \multicolumn{1}{l}{Best IntraMD} & \multicolumn{1}{l}{Best InterMD} & \multicolumn{1}{l}{Best EBCCB} \\ \midrule
IntraMD (cohesion)          & 205.173\%    & 151.335\%    & 55.011\%   \\
InterMD (coupling)          & 3.567\%      & 3.656\%      & 1.226\%    \\
EBCCB                       & 0.168\%      & 0.916\%      & 1.667\%    \\
\#Class change refactorings & 170          & 138          & 67         \\ \bottomrule
\end{tabular}
\end{table}

\begin{table}[H]
\caption{Relative improvement of best solutions for each optimization variable}
\label{bestresults}
\begin{tabular}{@{}lrrr@{}}
\toprule
                            & \multicolumn{1}{l}{Best IntraMD} & \multicolumn{1}{l}{Best InterMD} & \multicolumn{1}{l}{Best EBCCB} \\ \midrule
IntraMD (cohesion)          & 530.404\%    & 322.315\%    & 55.010\%   \\
InterMD (coupling)          & 1.204\%      & 6.041\%      & 1.226\%    \\
EBCCB                       & N/A          & -8.102\%     & 1.667\%    \\
\#Class change refactorings & 418          & 244          & 67         \\ \bottomrule
\end{tabular}
\end{table}
