# Supplementary material for: Search-Based Software Re-Modularization: A Case Study at Adyen
Source: arXiv:2102.00701 source file (2021-04-09)
Supplement: Supplementary file 2 [file appendix.tex]

\section{\label{cha:glossary}Glossary}

\subsection{Terminology}
In this subsection we give an overview of frequently used terms and
abbreviations.

\begin{itemize}
\item \textbf{Codebase}: The entire source code of a certain piece of software.

\item \textbf{Dependency structure}: The dependency structure is the total picture that arises from the dependencies from class to class. The way these classes are divided into modules results in dependencies from module to module. Both of these dependency levels can be represented with directed graphs. (see subsection\ref{sec:depstruc})

\item \textbf{(software/code) Architecture}: The structure of a piece of software or codebase. In this thesis, the term is often used to refer to the dependency structure in particular.

\item \textbf{Modularization}: The problem of dividing classes into modules in such a way that a good module structure is achieved. Re-modularization is the same problem, but from an already existing modularization, preferably with not too many changes.

\item \textbf{Cohesion}: An abstract concept representing how well a piece of code fits together. (see subsection \ref{sec:cohe})

\item \textbf{Coupling}: An abstract concept representing how interconnected a piece of code is. (see subsection \ref{sec:coup})

\item \textbf{IntraMD}: Intra Module Dependencies. The metric used in to represent cohesion. It is measured by the number of class depenencies in a module divided by the number of possible ones, summed for each module. 

\item \textbf{InterMD}: Inter Module Dependencies. The metric used in to represent coupling. It is measured by the number of module dependencies.

\item \textbf{CCP}: The Common Closure Principle \cite{Martin2003}. This is measured by the number of pairs of classes changed in the same commit over a set period of time.

\item \textbf{CRP}: The Common Reuse Principle \cite{Martin2003}. This is measured by the number of pairs of classes which are both in the same module and used by the same class, per class.

\item \textbf{(EA) Evolutionary Algorithm}: An optimization algorithm based on the concept of evolution. It contains some sort of population made of solutions, which procreate and mutate to form new solutions. The fittest solutions, which are the ones that optimize the problem the best, are allowed to procreate and mutate with the goal of finding fitter solutions.

\item \textbf{(MOEA) Multi-Objective Evolutionary Algorithm}: A type of evolutionary algorithm that optimizes for more than one value at the same time. In this type of algorithm, there is more than one "optimal" solution, often described as the pareto-front.

\item \textbf{Enterprise software}: Software made specifically to satisfy the needs of an organization. Often used in a way to emphasize the size/scale of the software.

\item \textbf{Build cost}: The cost of building a module, expressed in time. 

\item \textbf{Dead code}: Code that has not been used and changed in a while, and is not part of future plans.

\item \textbf{Transitive coupling / transitive dependencies}: If module M1 depends on module M2, and module M2 depends on module M3, M1 is said to be transitively coupled to / transitively dependent on module M3.

\item \textbf{Caching}: In this thesis caching refers to module build caching specifically. Module build caching is often used in enterprise-level software, especially in monolithic repositories. When a module is built, the built state is saved and shared so that any developer that needs the same state of the module does not have to build it. This process saves a lot of time for developers, whenever they want to run their code.

\item \textbf{Transitive cache breaks}: When some part of the code in a module is changed, its cache is broken. Due to this module being rebuilt, all the modules using this module also need to be rebuilt. This causes a cascading effect through the module dependency structure of cache breaks.

\item \textbf{(EBCCB) Estimated Build Cost of module Cache Breaks}: The new metric introduced in this thesis representing weighed transitive coupling. For further explanation see subsection \ref{EBCCB}.
\end{itemize}

\section{Interview}\label{appendix:interview}
\subsection{Interview Questions}
\begin{itemize}
\item Interviewee is given an explanation of the interview, the goal of the research, and that they are going to review a part of a solution generated by the algorithm.

\item How many years of experience in software development do you have?

\item How many years have you worked at Adyen?

\item How well would you say that you grasp the module to module dependency structure of the entire codebase, on a scale from 0 to 10?

\item How well would you say that you grasp the module to module dependency structure around \textit{the module the suggestion's classes are from}, on a scale from 0 to 10?

\item The interviewee is shown the suggestion and it is explained why this is an improvement in terms of the metrics.

\item Would you consider this suggestion to be a good change, meaning it has an overall positive impact on the codebase?

\item (If the interviewee does not give clear reasoning) Could you explain your reasoning for the previous answer?

\item (If the interviewee deems the suggestion to be good) How important would you rate this change in terms of severity and priority, on scales of 0 to 10? 

\item Has this change given you an idea on how to improve the code structure in this area of the code?
\end{itemize}

\subsection{Interview answers}

\begin{enumerate}[D1]
\item \textbf{How well would you say that you grasp the module dependency structure of the codebase?}

7/10

\noindent \textbf{How well would you say that you grasp the module dependency structure of the module C1 is in?}

7/10

\noindent \textbf{Would you consider this C1 to be a good change, meaning it has an overall positive impact on the codebase?}

\noindent \textbf{C1}: consists of moving one class to a new module. D1 deemed it to be a bad move. Logically the class fits in the module it is in, and moving just this class to a new module would make it too granular.

\noindent \textbf{Has this suggestion given you an idea on how to improve the code structure in this area of the code?}

This suggestion did reveal a very strange and possibly unnecessary dependency from this class to another module, causing multiple transitive dependencies. This is the cause of the EBCCB value impact of the suggestion.

\noindent \textbf{How well would you say that you grasp the module dependency structure of the module C2 is in?}

6/10

\noindent \textbf{Would you consider this C2 to be a good change, meaning it has an overall positive impact on the codebase?}

\noindent \textbf{C2}: consists of moving 2 classes to separate new modules, and 2 to existing modules. D1 verified that this move is good, however, there are better modules to move these classes to. Making modules for one class is again too granular, and there exist fitting modules for these 2 classes. Also, one of the classes that is moved to an existing module should be moved to a different one to follow design principles. 

\noindent \textbf{How important would you rate this change in terms of severity (impact relative to effort), and priority (compared to the day to day development tasks), on a scale from 0 to 10?}

Severity: 4/10

Priority: 7/10 

\item \textbf{How well would you say that you grasp the module dependency structure of the codebase?}

6/10

\noindent \textbf{How well would you say that you grasp the module dependency structure of the module C3 is in?}

6/10

\noindent \textbf{Would you consider this C3 to be a good change, meaning it has an overall positive impact on the codebase?}

\noindent \textbf{C3}: consists of moving one class to a different module. D2 deemed this to be a good move. The class is not used and is not using anything in its current module. However, there is a future plan for the module it is moved to that would make it not fit. Given this information, it would be better to construct a new module specifically for this class and related functionality.

\noindent \textbf{How important would you rate this change in terms of severity (impact relative to effort), and priority (compared to the day to day development tasks), on a scale from 0 to 10?}

Severity: 4/10

Priority: 4/10

\item \textbf{How well would you say that you grasp the module dependency structure of the codebase?}

7/10

\noindent \textbf{How well would you say that you grasp the module dependency structure of the module C4 is in?}

7/10

\noindent \textbf{Would you consider this C4 to be a good change, meaning it has an overall positive impact on the codebase?}

\noindent \textbf{C4}: consists of moving 1 class to a new module, and 1 class to a different module. D3 deemed this suggestion to be bad and good at the same time. The suggestion is bad because the class that is moved to a new module is dead code causing unnecessary dependencies, so it would be better to delete it entirely. The move of the other class is good in some sense, as it has been the part of an ongoing discussion where a group of developers is advocating for moving multiple classes to the module this class is suggested to be moved to. However, another group of developers says it is where it should be. What has become clear by this interview is that the class does not adhere to the design pattern properly. Before a move would be made, the class should be fixed first.

\noindent \textbf{How important would you rate this change in terms of severity (impact relative to effort), and priority (compared to the day to day development tasks), on a scale from 0 to 10?}

Severity: 2/10

Priority: 2/10

\item \textbf{How well would you say that you grasp the module dependency structure of the codebase?}

4/10

\noindent \textbf{How well would you say that you grasp the module dependency structure of the module C5 is in?}

5/10

\noindent \textbf{Would you consider this C5 to be a good change, meaning it has an overall positive impact on the codebase?}

\noindent \textbf{C5}: consists of moving 2 classes to a different module. D7 was also interviewed on this suggestion. D4 saw this as a bad change. One class is not necessarily in the wrong place. D4 is unsure about the other class, noting that it feels out of place. The module they are moved to is unfitting for both.

\noindent \textbf{Has this suggestion given you an idea on how to improve the code structure in this area of the code?}

No, no specific ideas.

\item \textbf{How well would you say that you grasp the module dependency structure of the codebase?}

3/10

\noindent \textbf{How well would you say that you grasp the module dependency structure of the module C6 is in?}

5/10

\noindent \textbf{Would you consider this C6 to be a good change, meaning it has an overall positive impact on the codebase?}

\noindent \textbf{C6}: consists of one class being moved to a new module. D5 verified this to be a bad move. The class has been superseded by another piece of functionality D5 wrote, so it should be removed and usages transferred, instead of being moved to a new module.

\noindent \textbf{Has this suggestion given you an idea on how to improve the code structure in this area of the code?}

Remove the class and transfer the usages to the other functionality.

\item \textbf{How well would you say that you grasp the module dependency structure of the codebase?}

5/10

\noindent \textbf{How well would you say that you grasp the module dependency structure of the module C7 is in?}

9/10

\noindent \textbf{Would you consider this C7 to be a good change, meaning it has an overall positive impact on the codebase?}

\noindent \textbf{C7}: consists of one class being moved to another module. D6 said this move makes sense in the current state of the code, however, there are structural plans for new functionality that will use the moved class, making the suggestion bad. 

\noindent \textbf{Has this suggestion given you an idea on how to improve the code structure in this area of the code?}

It has shown the module to be a catch-all, so splitting it would be an improvement.

\noindent \textbf{How well would you say that you grasp the module dependency structure of the module C8 is in?}

4/10

\noindent \textbf{Would you consider this C8 to be a good change, meaning it has an overall positive impact on the codebase?}

\noindent \textbf{C8}: consists of one class being moved to another (very closely related) module. D6 states the class fits in both modules, so given the algorithm's metrics, the move is good. 

\noindent \textbf{How important would you rate this change in terms of severity (impact relative to effort), and priority (compared to the day to day development tasks), on a scale from 0 to 10?}

Severity: 2/10

priority: 2/10

\item \textbf{How well would you say that you grasp the module dependency structure of the codebase?}

5/10

\noindent \textbf{How well would you say that you grasp the module dependency structure of the module C5 is in?}

8/10

\noindent \textbf{Would you consider this C5 to be a good change, meaning it has an overall positive impact on the codebase?}

\noindent \textbf{C5}: consists of moving 2 classes to a different module. D4 was also interviewed on this suggestion. D7 states that the first class should be moved according to the suggestion as it fits better in the suggested module. The second class doesn't fit its current module, partly due to it holds too much differing functionality. It should be fixed first, but in its current state, the move would be good. 

\noindent \textbf{How important would you rate this change in terms of severity (impact relative to effort), and priority (compared to the day to day development tasks), on a scale from 0 to 10?}

Severity: 8/10

Priority: 3/10

\item \textbf{How well would you say that you grasp the module dependency structure of the codebase?}

8/10

\noindent \textbf{How well would you say that you grasp the module dependency structure of the module C9 is in?}

8/10

\noindent \textbf{Would you consider this C9 to be a good change, meaning it has an overall positive impact on the codebase?}

\noindent \textbf{C9}: consists of moving 2 classes to different new modules. D8 determined this to be bad. One of the classes is dead code, so instead it should be removed. The other should be moved, but not to a new module, as it fits some existing modules already.

\noindent \textbf{Has this suggestion given you an idea on how to improve the code structure in this area of the code?}

Yes, remove the dead code and also move the other class to a fitting existing module

\noindent \textbf{How well would you say that you grasp the module dependency structure of the module C10 is in?}

9/10

\noindent \textbf{Would you consider this C10 to be a good change, meaning it has an overall positive impact on the codebase?}

\noindent \textbf{C10}: consists of moving 1 class to a different module. D8 stated that this move is bad, as the class fits its current module and does not fit the suggested module. However, looking at this suggestion has shown that something is off about the structure around and the usage of this class.

\noindent \textbf{Has this suggestion given you an idea on how to improve the code structure in this area of the code?}

Fix the usage of this class.

\item \textbf{How well would you say that you grasp the module dependency structure of the codebase?}

4/10

\noindent \textbf{How well would you say that you grasp the module dependency structure of the module C11 is in?}

5/10

\noindent \textbf{Would you consider this C11 to be a good change, meaning it has an overall positive impact on the codebase?}

\noindent \textbf{C11}: consists of moving 1 class to a different module. D9 has verified this to be a good move, as it is only used in the suggested module and not in the one it is in. 

\noindent \textbf{How important would you rate this change in terms of severity (impact relative to effort), and priority (compared to the day to day development tasks), on a scale from 0 to 10?}

Severity: 7/10 

Priority: 4/10

\item \textbf{How well would you say that you grasp the module dependency structure of the codebase?}

4/10

\noindent \textbf{How well would you say that you grasp the module dependency structure of the module C12 is in?}

0/10

\noindent \textbf{Would you consider this C12 to be a good change, meaning it has an overall positive impact on the codebase?}

\noindent \textbf{C12}: consists of moving 1 class to a different module. D10 has stated that this move is bad, due to the suggested module being in a refactoring process with the goal of splitting it up. This class was moved to its current module in the process, but it's not the best place for it. A better option would be to take this class, related functionality from the suggested module, and related functionality which is in a different module and combine it into a new module. Looking into this also revealed that code from the class' module seems quite stale, so it should be looked into.

\noindent \textbf{Has this suggestion given you an idea on how to improve the code structure in this area of the code?}

Create a new module around the class and its related functionality.

\item \textbf{How well would you say that you grasp the module dependency structure of the codebase?}

3/10

\noindent \textbf{How well would you say that you grasp the module dependency structure of the module C13 is in?}

10/10

\noindent \textbf{Would you consider this C13 to be a good change, meaning it has an overall positive impact on the codebase?}

\noindent \textbf{C13}: consists of moving a package of 6 classes to a different module, and 1 other class to a new module. D11 confirmed the package move to be good. However, the other class should be removed instead of moved, because it is dead code.

\noindent \textbf{How important would you rate this change in terms of severity (impact relative to effort), and priority (compared to the day to day development tasks), on a scale from 0 to 10?}

Severity: 8/10 

Priority: 6/10

\end{enumerate}

\section{Figures \& Tables}\label{appendix:figures}

\subsection{LOC correlation with build costs}
In the Figures, \ref{fig:LOCCompile} and \ref{fig:LOCjar}, the correlation between build tasks and LOC, and the formula achieved through regression can be seen. The function shown was achieved by feeding a function in the following form into the \textit{optimize.curve\_fit} function of python package \textit{scipy}, and using the relative error instead of absolute:
\begin{equation}
f(x) = a * log_{10}(x)^b + c
\end{equation}

\begin{figure}[H]
\centering
\includegraphics[width = \textwidth]{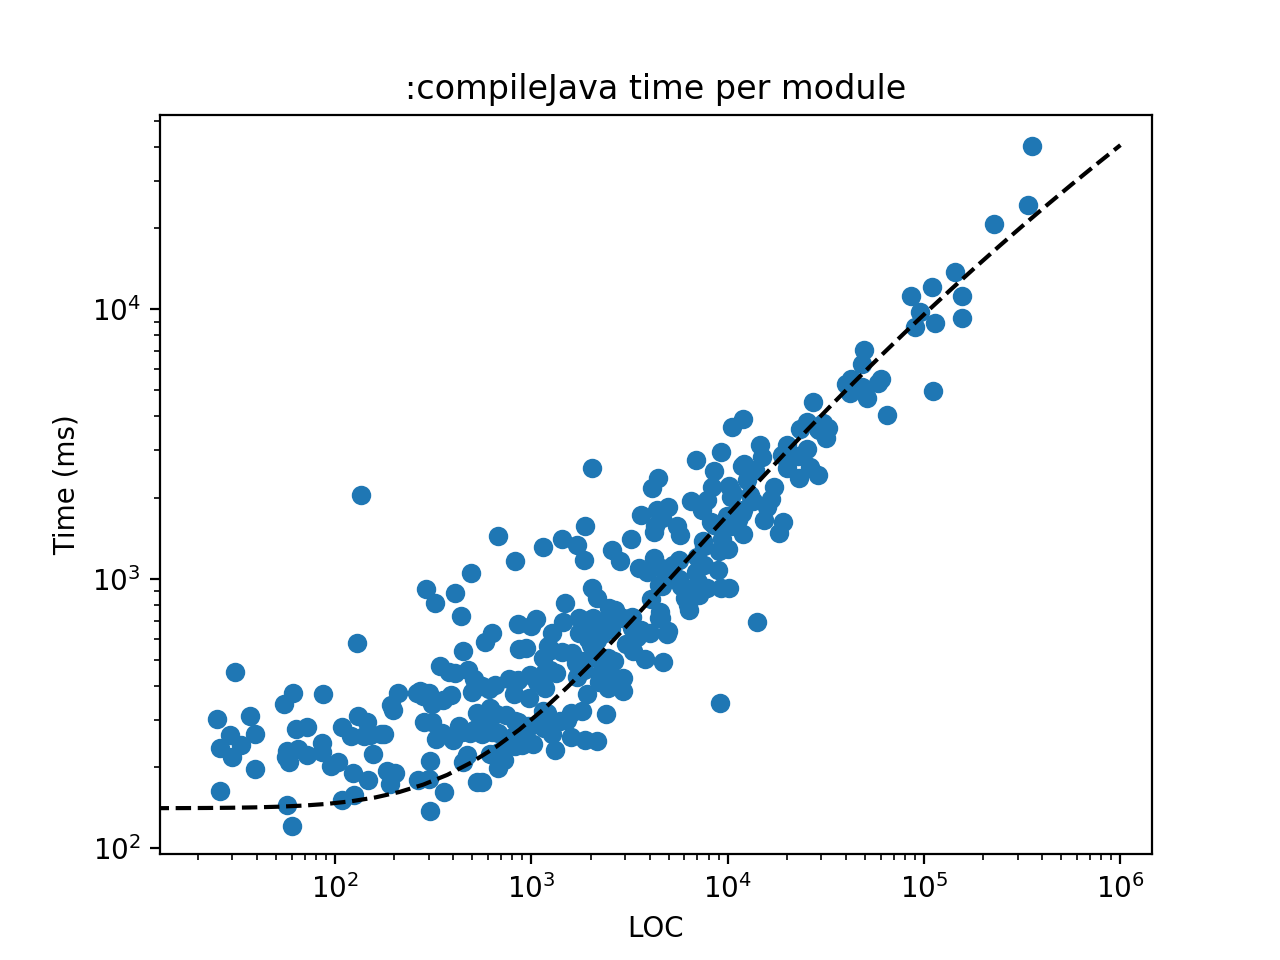}
\caption{The runtime of a compile Java task relative to the lines of code in the module}
\label{fig:LOCCompile}
\end{figure}

\begin{figure}[H]
\centering
\noindent
\includegraphics[width = \textwidth]{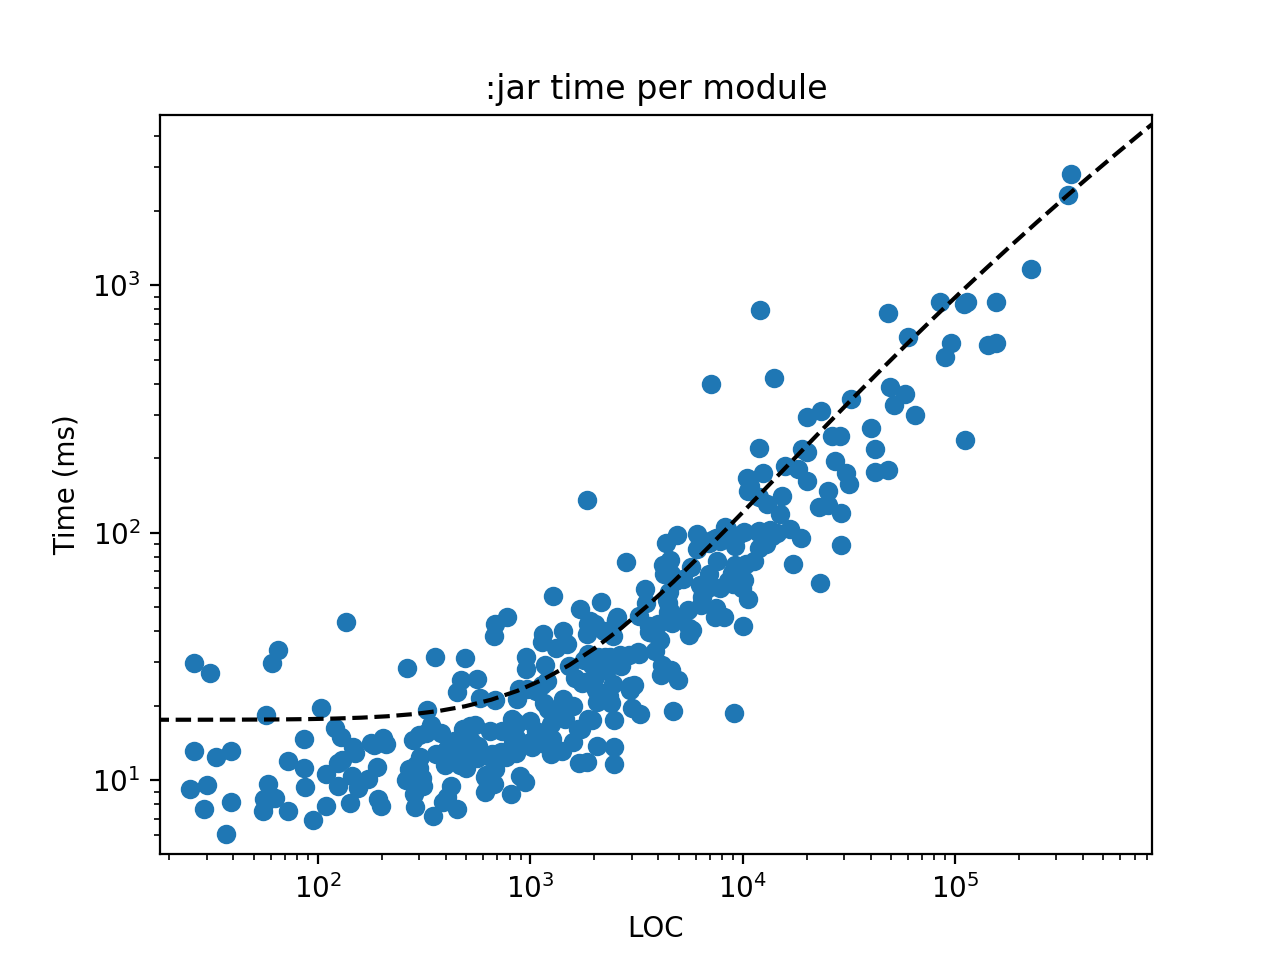}
\caption{The runtime of a jar task relative to the lines of code in the module}
\label{fig:LOCjar}
\end{figure}

\subsection{Optimization variable tweaking results}\label{appendix:optvartweak}
The results can be seen in Table \ref{optvartweak} \& \ref{optvartweak2}. These tables contain the highest amount of generations that was achieved in the 5 runs per configuration, the average amount of generations, the best value of each optimization variable for solutions in all runs, and the average value of the best values per optimization variable per run. Note that all optimization variables use the existing architecture as the 0 point and negative values show improvements (the values of CCP, CRP, and Intra Module Coupling are flipped).
The optimization variable configurations are as follows:

\begin{enumerate}
\item IntraMD, InterMD, EBCCB, \# Changes

A combination including all aspects optimized for, with only one Cohesion metric.

\item IntraMD, InterMD

This combination has been used in modularization research before\cite{Harman2002}. It is included as a baseline to show the value of EBCCB as an optimization variable, and other combinations tested.

\item InterMD, CRP, CCP

A combination that also optimizes for Coupling and Cohesion, with CCP and CRP used for Cohesion.

\item IntraMD, InterMD, EBCCB, CCP, CRP, \# Changes

This combination uses all optimization variables to show its performance compared to the other combinations.

\item IntraMD, EBCCB

This combination optimizes for one of the types of Cohesion and the newly proposed metric, which is also used here as a type of coupling.

\item IntraMD, InterMD, \# Changes

A combination to show the effect of optimizing for the number of classes moved compared to the often used cohesion/coupling combination. 

\item IntraMD, CCP, CRP

The combination of only Cohesion optimization variables. It's included to show the effect of ignoring Coupling metrics.

\item InterMD, EBCCB

This combination of coupling and the newly introduced metric. It's included to show the effect of ignoring Cohesion metrics.

\item InterMD, CCP, CRP, EBCCB, \# Changes

A similar combination to the first one, using the other Cohesion metrics.

\item IntraMD, EBCCB, \# Changes

The same combination as \#5, with the number of classes moved. This shows the effect of optimizing or ignoring the number of changes with these other optimization variables.

\item CCP, CRP, EBCCB, \# Changes

A similar combination of optimization variables as the previous combination, with the other Cohesion optimization variables.
\end{enumerate}

From the tested configurations, we concluded that configuration 1 is the best choice, as it shows a consistent improvement across the different variables tested, with the best improvement in some cases. It also performs well in terms of number of generations reached.

\begin{landscape}
\begin{table}[]
\caption{Optimization variable tweaking results (1/2)}
\label{optvartweak}
\resizebox{1.5\textwidth}{!}{%
\begin{tabular}{@{}rrrrrrrrr@{}}
\toprule
\multicolumn{1}{l}{Configuration} & \multicolumn{1}{l}{Highest \# generations} & \multicolumn{1}{l}{Average \# generations} & \multicolumn{1}{l}{IntraMD best} & \multicolumn{1}{l}{IntraMD average} & \multicolumn{1}{l}{CCP best} & \multicolumn{1}{l}{CCP average} & \multicolumn{1}{l}{CRP best} & \multicolumn{1}{l}{CRP average} \\ \midrule
1                    & 3291                                       & 2923                                       & -201.19203                       & -188.056636                         & -3                           & -0.6                            & -358.5                       & -144.3                          \\
2                    & 1627                                       & 1332.4                                     & -353.89275                       & -303.321648                         & 500                          & 2528.7                          & -213.5                       & 4953.2                          \\
3                    & 350                                        & 276.6                                      & -9.44654                         & -7.567176                           & \textbf{-5143.5}             & \textbf{-4196.1}                & -45810.5                     & -37781.6                        \\
4                    & 1629                                       & 1451.2                                     & -155.68067                       & -136.209968                         & -359                         & -155.1                          & -2515                        & -1856.5                         \\
5                    & 3060                                       & 1682.6                                     & \textbf{-381.06114}              & -307.17393                          & 716                          & 2327.9                          & -323.5                       & 1379.7                          \\
6                    & 3422                                       & 3242.6                                     & -373.13179                       & \textbf{-349.270522}                & 0                            & 0                               & -87                          & -71.2                           \\
7                    & 246                                        & 227                                        & -86.35844                        & -77.499758                          & -4318.5                      & -3716                           & \textbf{-54467}              & \textbf{-42200.2}               \\
8                    & \textbf{6138}                              & \textbf{5700.8}                            & -4.82292                         & -3.562402                           & 14                           & 51.4                            & -120.5                       & -107.5                          \\
9                    & 994                                        & 479.2                                      & -9.1541                          & -8.104232                           & -4866                        & -3199                           & -44588.5                     & -28359.7                        \\
10                   & 3310                                       & 2981.2                                     & -181.89897                       & -176.163372                         & 0                            & 0                               & 0                            & 0                               \\
11                   & 401                                        & 332.4                                      & -9.30071                         & -6.689142                           & -3590.5                      & -3225.6                         & -48990                       & -38548.4                        \\ \bottomrule
\end{tabular}%
}
\end{table}
\end{landscape}

\begin{landscape}
\begin{table}[]
\caption{Optimization variable tweaking results (2/2)}
\label{optvartweak2}
\resizebox{1.5\textwidth}{!}{%

\begin{tabular}{@{}rrrrrrr@{}}
\toprule
\multicolumn{1}{l}{Configuration} & \multicolumn{1}{l}{Highest \# generations} & \multicolumn{1}{l}{Average \# generations} & \multicolumn{1}{l}{InterMD best} & \multicolumn{1}{l}{InterMD average} & \multicolumn{1}{l}{EBCCB best} & \multicolumn{1}{l}{EBCCB average} \\ \midrule
1                    & 3291                                       & 2923                                       & \textbf{-10}                     & -9.4                                & \textbf{-8868.766327}          & -7249.249941                      \\
2                    & 1627                                       & 1332.4                                     & \textbf{-10}                     & -7.2                                & -89.75918085                   & 15462.80009                       \\
3                    & 350                                        & 276.6                                      & -8                               & -5.6                                & 37484.10431                    & 345335.6063                       \\
4                    & 1629                                       & 1451.2                                     & \textbf{-10}                     & -9                                  & \textbf{-8868.766327}          & -5998.596233                      \\
5                    & 3060                                       & 1682.6                                     & 74                               & 265.2                               & -8696.175143                   & -6858.179237                      \\
6                    & 3422                                       & 3242.6                                     & -9                               & -8.4                                & -1855.888897                   & -1662.609525                      \\
7                    & 246                                        & 227                                        & 93                               & 132.8                               & 999999                         & 999999                            \\
8                    & \textbf{6138}                              & \textbf{5700.8}                            & \textbf{-10}                     & \textbf{-9.8}                       & \textbf{-8868.766327}          & \textbf{-8497.082381}             \\
9                    & 994                                        & 479.2                                      & \textbf{-10}                     & -3.6                                & \textbf{-8868.766327}          & -1846.221569                      \\
10                   & 3310                                       & 2981.2                                     & 0                                & 0                                   & -8146.341455                   & -5516.492598                      \\
11                   & 401                                        & 332.4                                      & -7                               & -1.4                                & -2183.037166                   & -767.415869                       \\ \bottomrule
\end{tabular}%
}
\end{table}
\end{landscape}

\subsection{Parameter tuning results}\label{appendix:paramtune}
This subsection holds the results of the parameter tuning runs. The results can be seen in the tables in this subsection. One table exists per tweaked parameter. The tables show the highest amount of generations that was achieved in the 5 runs per parameter, the average amount of generations, the best value of each used optimization variable for all solutions in all runs, and the average value of the best values per used optimization variable per run.

\noindent The default settings for all parameters are as follows:
\begin{itemize}
\item Population size = 500
\item Mutation chance = 0.5
\item Both mutation operators are used with equal probability
\item Constraint breaks are ignored
\item Duplicates are deleted
\item The crossover operator that conserves building blocks is used
\item An elite archive is not used
\end{itemize}

\noindent The options the parameters are tweaked for are as follows, with the optimal options in bold:

\begin{itemize}
\item Population size = \{50, 100, 200, \textbf{500}, 1000, 2000\}
\item Mutation chance = \{0.05, 0.1, 0.2, \textbf{0.5}\}
\item The optimal ratio of mutation operator usage = \{0.25, \textbf{0.50}, 0.75\}
\item Whether solutions that break constraints are punished, repaired or whether \textbf{constraint breaks are ignored}
\item How duplicates should be handled; by ignoring them, \textbf{deleting them} or mutating them
\item Which crossover operator is used; the single-point operator or \textbf{the one that tries to preserve building blocks}.
\item Whether an elite archive is used.
\end{itemize}

Note that for both population size and elite archive there was no clear optimal choice, so we decided to go for parameter values that have a balanced trade-off in performance and solution diversity. This resulted in a population size of 500, and using an elite archive of the size of the population, as it doubled the number of unique solutions while barely impacting performance.

\begin{landscape}
\begin{table}[]
\caption{Mutation choice parameter tuning results}
\resizebox{1.5\textwidth}{!}{%

\begin{tabular}{@{}rrrrrrrrr@{}}
\toprule
\multicolumn{1}{l}{\begin{tabular}[c]{@{}l@{}}Mutation \\ Choice\end{tabular}} & \multicolumn{1}{l}{\begin{tabular}[c]{@{}l@{}}Highest \\ \# generations\end{tabular}} & \multicolumn{1}{l}{\begin{tabular}[c]{@{}l@{}}Average \\ \# generations\end{tabular}} & \multicolumn{1}{l}{\begin{tabular}[c]{@{}l@{}}IntraMD \\ best\end{tabular}} & \multicolumn{1}{l}{\begin{tabular}[c]{@{}l@{}}IntraMD \\ average\end{tabular}} & \multicolumn{1}{l}{\begin{tabular}[c]{@{}l@{}}InterMD \\ best\end{tabular}} & \multicolumn{1}{l}{\begin{tabular}[c]{@{}l@{}}InterMD \\ average\end{tabular}} & \multicolumn{1}{l}{EBCCB best} & \multicolumn{1}{l}{EBCCB average} \\ \midrule
0.25                          & 3047                                       & 2735.6                                     & -204.35977                       & -196.329108                         & -9                               & -9                                  & \textbf{-8868.766327}          & -7617.684572                      \\
0.5                           & 3379                                       & 3094.6                                     & \textbf{-241.85756}              & \textbf{-211.027916}                & \textbf{-10}                     & -9.2                                & \textbf{-8868.766327}          & \textbf{-8796.452694}             \\
0.75                          & \textbf{3439}                              & \textbf{3315.2}                            & -217.37067                       & -179.69686                          & \textbf{-10}                     & \textbf{-9.6}                       & \textbf{-8868.766327}          & -7504.235915                      \\ \bottomrule
\end{tabular}%
}
\end{table}
\end{landscape}

\begin{landscape}
\begin{table}[]
\caption{Mutation chance parameter tuning results}
\resizebox{1.5\textwidth}{!}{%

\begin{tabular}{@{}rrrrrrrrr@{}}
\toprule
\multicolumn{1}{l}{\begin{tabular}[c]{@{}l@{}}Mutation \\ Chance\end{tabular}} & \multicolumn{1}{l}{\begin{tabular}[c]{@{}l@{}}Highest \\ \# generations\end{tabular}} & \multicolumn{1}{l}{\begin{tabular}[c]{@{}l@{}}Average \\ \# generations\end{tabular}} & \multicolumn{1}{l}{\begin{tabular}[c]{@{}l@{}}IntraMD \\ best\end{tabular}} & \multicolumn{1}{l}{\begin{tabular}[c]{@{}l@{}}IntraMD \\ average\end{tabular}} & \multicolumn{1}{l}{\begin{tabular}[c]{@{}l@{}}InterMD \\ best\end{tabular}} & \multicolumn{1}{l}{\begin{tabular}[c]{@{}l@{}}InterMD \\ average\end{tabular}} & \multicolumn{1}{l}{EBCCB best} & \multicolumn{1}{l}{EBCCB average} \\ \midrule
0.05                          & 3485                                       & 3236.8                                     & -230.86222                       & -203.496192                         & \textbf{-10}                     & -9.2                                & -8507.19816                    & -8505.507435                      \\
0.1                           & 3349                                       & 3268.8                                     & -238.8507                        & -204.025204                         & -9                               & -9                                  & \textbf{-8868.766327}          & -8650.698277                      \\
0.2                           & \textbf{3514}                              & \textbf{3371}                              & -230.85718                       & -205.87951                          & \textbf{-10}                     & \textbf{-9.6}                       & -8507.19816                    & -7176.936307                      \\
0.5                           & 3379                                       & 3094.6                                     & \textbf{-241.85756}              & \textbf{-211.027916}                & \textbf{-10}                     & -9.2                                & \textbf{-8868.766327}          & \textbf{-8796.452694}             \\ \bottomrule
\end{tabular}%
}
\end{table}
\end{landscape}

\begin{landscape}
\begin{table}[]
\caption{Dealing with solutions that break constaints parameter tuning results}
\resizebox{1.5\textwidth}{!}{%

\begin{tabular}{@{}rrrrrrrrr@{}}
\toprule
\multicolumn{1}{l}{\begin{tabular}[c]{@{}l@{}l@{}}Constraint \\ Breaking \\ Solutions\end{tabular}} & \multicolumn{1}{l}{\begin{tabular}[c]{@{}l@{}}Highest \\ \# generations\end{tabular}} & \multicolumn{1}{l}{\begin{tabular}[c]{@{}l@{}}Average \\ \# generations\end{tabular}} & \multicolumn{1}{l}{\begin{tabular}[c]{@{}l@{}}IntraMD \\ best\end{tabular}} & \multicolumn{1}{l}{\begin{tabular}[c]{@{}l@{}}IntraMD \\ average\end{tabular}} & \multicolumn{1}{l}{\begin{tabular}[c]{@{}l@{}}InterMD \\ best\end{tabular}} & \multicolumn{1}{l}{\begin{tabular}[c]{@{}l@{}}InterMD \\ average\end{tabular}} & \multicolumn{1}{l}{EBCCB best} & \multicolumn{1}{l}{EBCCB average} \\ \midrule
ignore           & \textbf{3379}                              & \textbf{3094.6}                            & \textbf{-241.85756}              & \textbf{-211.027916}                & \textbf{-10}                     & \textbf{-9.2}                       & \textbf{-8868.766327}          & \textbf{-8796.452694}             \\
punish           & 2701                                       & 2472.6                                     & -191.06344                       & -179.100518                         & \textbf{-10}                     & -7.8                                & -8696.175143                   & -7312.543237                      \\
repair           & 2737                                       & 2604                                       & -168.18622                       & -159.756326                         & -9                               & -9                                  & \textbf{-8868.766327}          & -8723.575485                      \\ \bottomrule
\end{tabular}%
}
\end{table}
\end{landscape}

\begin{landscape}
\begin{table}[]
\caption{Dealing with duplicate solutions parameter tuning results}
\resizebox{1.5\textwidth}{!}{%

\begin{tabular}{@{}rrrrrrrrr@{}}
\toprule
\multicolumn{1}{l}{\begin{tabular}[c]{@{}l@{}}Dealing with \\ Duplicates\end{tabular}} & \multicolumn{1}{l}{\begin{tabular}[c]{@{}l@{}}Highest \\ \# generations\end{tabular}} & \multicolumn{1}{l}{\begin{tabular}[c]{@{}l@{}}Average \\ \# generations\end{tabular}} & \multicolumn{1}{l}{\begin{tabular}[c]{@{}l@{}}IntraMD \\ best\end{tabular}} & \multicolumn{1}{l}{\begin{tabular}[c]{@{}l@{}}IntraMD \\ average\end{tabular}} & \multicolumn{1}{l}{\begin{tabular}[c]{@{}l@{}}InterMD \\ best\end{tabular}} & \multicolumn{1}{l}{\begin{tabular}[c]{@{}l@{}}InterMD \\ average\end{tabular}} & \multicolumn{1}{l}{EBCCB best} & \multicolumn{1}{l}{EBCCB average} \\ \midrule
delete     & 3379                                       & 3094.6                                     & \textbf{-241.85756}              & -211.027916                         & \textbf{-10}                     & \textbf{-9.2}                       & \textbf{-8868.766327}          & \textbf{-8796.452694}             \\
ignore     & 3223                                       & 3011.4                                     & -236.8605                        & \textbf{-212.099254}                & \textbf{-10}                     & \textbf{-9.2}                       & \textbf{-8868.766327}          & -8651.261852                      \\
mutate     & \textbf{9438}                              & \textbf{9141.4}                            & -3                               & -2.60019                            & 0                                & 0                                   & 0                              & 0                                 \\ \bottomrule
\end{tabular}%
}
\end{table}
\end{landscape}

\begin{landscape}
\begin{table}[]
\caption{Crossover operator choice parameter tuning results}
\resizebox{1.5\textwidth}{!}{%

\begin{tabular}{@{}rrrrrrrrr@{}}
\toprule
\multicolumn{1}{l}{\begin{tabular}[c]{@{}l@{}}Crossover \\ Operator\end{tabular}} & \multicolumn{1}{l}{\begin{tabular}[c]{@{}l@{}}Highest \\ \# generations\end{tabular}} & \multicolumn{1}{l}{\begin{tabular}[c]{@{}l@{}}Average \\ \# generations\end{tabular}} & \multicolumn{1}{l}{\begin{tabular}[c]{@{}l@{}}IntraMD \\ best\end{tabular}} & \multicolumn{1}{l}{\begin{tabular}[c]{@{}l@{}}IntraMD \\ average\end{tabular}} & \multicolumn{1}{l}{\begin{tabular}[c]{@{}l@{}}InterMD \\ best\end{tabular}} & \multicolumn{1}{l}{\begin{tabular}[c]{@{}l@{}}InterMD \\ average\end{tabular}} & \multicolumn{1}{l}{EBCCB best} & \multicolumn{1}{l}{EBCCB average} \\ \midrule
building blocks    & 3379                                       & 3094.6                                     & \textbf{-241.85756}              & \textbf{-211.027916}                & \textbf{-10}                     & -9.2                                & \textbf{-8868.766327}          & \textbf{-8796.452694}             \\
single             & \textbf{4495}                              & \textbf{4010.4}                            & -78.84706                        & -73.8421                            & \textbf{-10}                     & \textbf{-9.6}                       & \textbf{-8868.766327}          & -8650.698277                      \\ \bottomrule
\end{tabular}%
}
\end{table}
\end{landscape}

\begin{landscape}
\begin{table}[]
\caption{Using an elite archive parameter tuning results}
\resizebox{1.5\textwidth}{!}{%

\begin{tabular}{@{}rrrrrrrrr@{}}
\toprule
\multicolumn{1}{l}{\begin{tabular}[c]{@{}l@{}}Use Elite \\ Archive\end{tabular}} & \multicolumn{1}{l}{\begin{tabular}[c]{@{}l@{}}Highest \\ \# generations\end{tabular}} & \multicolumn{1}{l}{\begin{tabular}[c]{@{}l@{}}Average \\ \# generations\end{tabular}} & \multicolumn{1}{l}{\begin{tabular}[c]{@{}l@{}}IntraMD \\ best\end{tabular}} & \multicolumn{1}{l}{\begin{tabular}[c]{@{}l@{}}IntraMD \\ average\end{tabular}} & \multicolumn{1}{l}{\begin{tabular}[c]{@{}l@{}}InterMD \\ best\end{tabular}} & \multicolumn{1}{l}{\begin{tabular}[c]{@{}l@{}}InterMD \\ average\end{tabular}} & \multicolumn{1}{l}{EBCCB best} & \multicolumn{1}{l}{EBCCB average} \\ \midrule
false                             & 3379                                       & 3094.6                                     & \textbf{-241.85756}              & \textbf{-211.027916}                & \textbf{-10}                     & -9.2                                & \textbf{-8868.766327}          & \textbf{-8796.452694}             \\
true                              & \textbf{3480}                              & \textbf{3251.6}                            & -220.85683                       & -202.05801                          & \textbf{-10}                     & \textbf{-9.6}                       & \textbf{-8868.766327}          & -7655.468213                      \\ \bottomrule
\end{tabular}%
}
\end{table}
\end{landscape}

\begin{landscape}
\begin{table}[]
\caption{Population size parameter tuning results}
\resizebox{1.5\textwidth}{!}{%

\begin{tabular}{@{}rrrrrrrrr@{}}
\toprule
\multicolumn{1}{l}{\begin{tabular}[c]{@{}l@{}}Population \\ Size\end{tabular}} & \multicolumn{1}{l}{\begin{tabular}[c]{@{}l@{}}Highest \\ \# generations\end{tabular}} & \multicolumn{1}{l}{\begin{tabular}[c]{@{}l@{}}Average \\ \# generations\end{tabular}} & \multicolumn{1}{l}{\begin{tabular}[c]{@{}l@{}}IntraMD \\ best\end{tabular}} & \multicolumn{1}{l}{\begin{tabular}[c]{@{}l@{}}IntraMD \\ average\end{tabular}} & \multicolumn{1}{l}{\begin{tabular}[c]{@{}l@{}}InterMD \\ best\end{tabular}} & \multicolumn{1}{l}{\begin{tabular}[c]{@{}l@{}}InterMD \\ average\end{tabular}} & \multicolumn{1}{l}{EBCCB best} & \multicolumn{1}{l}{EBCCB average} \\ \midrule
50                                  & \textbf{19744}                             & \textbf{18392}                             & \textbf{-413.53268}              & \textbf{-362.800888}                & -9                               & -8.4                                & -8696.175143                   & -8541.220927                      \\
100                                 & 13333                                      & 11722.8                                    & -365.02763                       & -341.461612                         & -9                               & -8.4                                & \textbf{-8868.766327}          & -8688.493674                      \\
200                                 & 8253                                       & 7671.2                                     & -330.70093                       & -288.728334                         & \textbf{-10}                     & -8.6                                & -8696.175143                   & -8501.486691                      \\
500                                 & 3379                                       & 3094.6                                     & -241.85756                       & -211.027916                         & \textbf{-10}                     & \textbf{-9.2}                       & \textbf{-8868.766327}          & \textbf{-8796.452694}             \\
1000                                & 1363                                       & 1201.8                                     & -128.85548                       & -110.552806                         & \textbf{-10}                     & \textbf{-9.2}                       & \textbf{-8868.766327}          & -8577.821069                      \\
2000                                & 407                                        & 362.8                                      & -53.84141                        & -50.14562                           & \textbf{-10}                     & \textbf{-9.2}                       & \textbf{-8868.766327}          & -8723.011911                      \\ \bottomrule
\end{tabular}%
}
\end{table}
\end{landscape}

\section{Pseudocode Estimated Build Cost of module Cache Breaks Difference}\label{buildcostPseudo}
This appendix section contains the pseudocode that represents the code used to calculate the EBCCB metric.

\begin{algorithm}
\caption{Functionality used to calculate the difference in EBCCB value between the given solution and the base solution}
\begin{algorithmic}[1]
\Function{CalculateEBCCBDiff}{$G, Sol, TDeps, ROCpM, LOCpM, ModsCT$}

	\State $G = (V,E)$ \Comment{\parbox[t]{.5\linewidth}{Graph representing module dependencies, weighted by the number of class dependencies}
	\State $Sol$ \Comment{The solution}}
	\State $ROCpM$ \Comment{\parbox[t]{.5\linewidth}{The rate of change per module, based on commit history,  adjusted for changes in this solution}}
	\State $LOCpM$ \Comment{\parbox[t]{.5\linewidth}{the number of lines of code per module adjusted for changes in this solution}}
	\State $ModsCT$ \Comment{\parbox[t]{.5\linewidth}{A mapping from module to module, containing the number of times they were changed together, used to correct the ROC to accurately represent the number of cache breaks}}

	\State $TDeps$ \Comment{\parbox[t]{.5\linewidth}{A mapping from each module to all its transitive dependencies}}

	\State $Er \gets \emptyset$ \Comment{Set of removed edges}
	\State $Ea \gets \emptyset$ \Comment{Set of added edges}

	\State $Ea, Er \gets $\Call{GetChangedEdges}{$G, Sol$}

	\State $TDa \gets \emptyset$ \Comment{\parbox[t]{.5\linewidth}{Transitive module dependencies that have been added by the changes in the solution}}
	\State $TDr \gets \emptyset$ \Comment{\parbox[t]{.5\linewidth}{Transitive module dependencies that have been removed by the changes in the solution}}

	\State $TDa, TDr \gets $\Call{GetChangedTransDeps}{$G, Ea, Er, TDeps$}

	\State $EBCCB \gets$\Call{CalcEBCCB}{$TDa, TDr, ROCpM, LOCpM, ModsCT$}

	\Return $EBCCB$

\EndFunction
\end{algorithmic}
\end{algorithm}

\begin{algorithm}
\caption{Determines the module dependencies (edges) which are added or removed by the class moves of a solution}

\begin{algorithmic}[1]
\Function{GetChangedEdges}{$G, Sol$}
	\State $Ea, Er \gets \emptyset$
	\State $Ec \gets Map$ \Comment{Map of changed edges to their weights}

	\For{$class$ in $Sol.changes$}
		\State $Ec \gets Ec \cup module\_edge\_changes$ \Comment{\parbox[t]{.5\linewidth}{Add every module edge affected by this class change to Ec, and weigh them by the effect of the change on the edge weight}}
	\EndFor

	\For{$edge$ in $Ec$}
		\State \Comment{\parbox[t]{.5\linewidth}{If the edge is a newly introduced one}}
		\If{$edge\notin	G.E$ AND $Ec.edge > 0$} 
			\State $Ea \gets Ea \cup edge$
		\EndIf
		\State \Comment{\parbox[t]{.5\linewidth}{If all class dependencies between the 
		vertices of this edge no longer exist}}
		\If{$edge\in G.E$ AND $G.E.edge - Ec.edge == 0$} 
			\State $Er \gets Er \cup edge$
		\EndIf		
	\EndFor

	\Return $Ea, Er$
\EndFunction

\end{algorithmic}
\end{algorithm}

\begin{algorithm}
\caption{Finds the changed transitive module dependencies which are caused by the added and removed module dependencies of a solution}
\begin{algorithmic}[1]
\Function{GetChangedTransDeps}{$G, Er, Ea, TDeps$}
	\State $vToCheck \gets trans\_deps\_Er\_Ea$ \Comment{\parbox[t]{.5\linewidth}{All transitive dependencies of destination vertices in Er and Ea}} 
	\State $knownRevDeps \gets Map$ \Comment{\parbox[t]{.5\linewidth}{A mapping from modules to their known transitive reverse dependencies}}
	\State $Vv \gets \emptyset$ \Comment{Visited vertices}
	\State $Vcircular \gets \emptyset$ \Comment{\parbox[t]{.5\linewidth}{Nodes that can be found through its own transitive reverse dependencies}}
	\State $circular \gets false$
	\State $res \gets Map$ \Comment{\parbox[t]{.5\linewidth}{Mapping of all checked vertices to a mapping of the found reverse dependencies and whether they are reachable or not}}

	\State $TDa, TDr \gets \emptyset$

	\For{$v$ in $vToCheck$}
		\State $vRes, thisCircular, knownRevDeps, Vcircular \gets$ \Call{RecursiveEdgeCheck}{$v, G, Er, Ea, Vv,$ $
			knownRevDeps, reachable \gets true,$ $edgePrevExists \gets 
			true, Vcircular$}
		\State $circular \gets circular$ OR $thisCircular$ 
		\State $res.v \gets vRes$ 
	\EndFor

	\State $res \gets updated\_res$ \Comment{\parbox[t]{.5\linewidth}{Update the reachable vertices of each vertex in Vcircular with the reachable vertices of all other vertices in Vcircular}}
	\State $res \gets updated\_res$ \Comment{\parbox[t]{.5\linewidth}{Update the reachable vertices of all vertices that can reach a vertex in Vcircular with that vertex' reachable vertices}}

	\For{$v$ in $res$}
		\For{$vr$ in $res.v$}
		\If{$res.v.vr == true$ AND $v \notin TDeps.vr$}
			\State $TDa \gets TDa \cup (vr,v)$
		\ElsIf{$res.v.vr == false$ AND $v \in TDeps.vr$}
			\State $TDr \gets TDr \cup (vr,v)$
		\EndIf
		\EndFor
	\EndFor

	\Return $TDa, TDr$
\EndFunction

\end{algorithmic}
\end{algorithm}

\begin{algorithm}
\caption{Recusively checks the reverse transitive dependencies of a module (vertex). Returns the found dependencies, whether they are reachable, whether there exists a circular dependency and which modules are part of that circle. It saves the results for each modules in a dynamic programming way.}
{\footnotesize
\begin{algorithmic}[1]
\Function{RecursiveEdgeCheck}{$v, G, Er, Ea, Vv,
			knownRevDeps, reachable, edgePrevExists, Vcircular$}
	\State $vRes \gets \emptyset$
	\State $thisCircular \gets false$

	\If{$v \in Vv$} \Comment{A potential circular dependency is found}
		\State $vRes \gets {v: edgeToPreviousExists}$
		\State $thisCircular \gets reachable$
		\State $Vcircular \gets Vcircular \cup v$
		\State\Return $vRes, thisCircular, knownRevDeps, Vcircular$

	\EndIf

	\If{$v \in knownRevDeps$} \Comment {v's reverse dependencies are known}
		\State\Return $knownRevDeps.v.vRes, knownRevDeps.v.thisCircular, knownRevDeps, Vcircular$
	\EndIf

	\State $Vv \gets Vv \cup v$

	\State $revDeps \gets $ all $vo$ where $(vo, v) \in G.E $ OR $ (vo, v) \in Ea$

	\For{$vo \in revDeps$} \Comment{Recursively check all reverse dependencies}
		\State $depExists \gets (vo, v) \notin Er$

		\If{$depExists$}
			\State $voRes, otherCircular, oknownRevDeps, oVcircular \gets$ \Call{RecursiveEdgeCheck}{$vo, G, Er, Ea, Vv,
			knownRevDeps, reachable, edgePrevExists \gets true, Vcircular$}
			\State $vRes.vo \gets true$
			\For{$voo \in voRes$}
				\If{$voo == v$}
					\State $Vcircular \gets Vcircular \cup v$
				\EndIf
				\If{$voo \notin vRes$}
					\State $vRes.voo \gets voRes.voo$
				\Else
					\State $vRes.voo \gets vRes.voo$ OR $voRes.voo$
				\EndIf

			\EndFor

		\Else
			\State $voRes, otherCircular, oknownRevDeps, oVcircular \gets$ \Call{RecursiveEdgeCheck}{$vo, G, Er, Ea, Vv,
			knownRevDeps, reachable \gets false, edgePrevExists \gets false, Vcircular$}
			\If{$vo \notin vRes$}
				\State $vRes.vo \gets false$
			\EndIf
			\For{$voo \in voRes$}
				\If{$voo \notin vRes$}
					\State $vRes.voo \gets false$
				\EndIf
			\EndFor

		\EndIf

		\State $thisCircular \gets otherCircular$ OR $thisCircular$

	\EndFor

	\If{$v \notin vRes$} \Comment{Add reachability of v for the previous vertex}
		\State $vRes.v \gets edgePrevExists$
	\Else
		\State $vRes.v \gets vRes.v \cup edgePrevExists$
	\EndIf

	\State $Vv.remove(v)$
	\State $knownRevDeps.v \gets vRes, thisCircular$

	\Return $vRes, thisCircular, knownRevDeps, Vcircular$
\EndFunction

\end{algorithmic}
}
\end{algorithm}

\begin{algorithm}
\caption{Calculates the EBCCB metric (relative) value, given the changed transitive dependencies, Rate of Change per module, Lines of Code per module and the amount of times module pairs are changed together.}
\begin{algorithmic}[1]
\Function{CalcEBCCB}{$TDa, TDr, ROCpM, LOCpM, ModsCT$}
	\State $costChange \gets 0$
	\For{$(v1,v2) \in TDa$}
		\State $cacheBreaks \gets ROCpM.v2 - ModsCT.v1.v2$
		\State $cost \gets $\Call{LOCtoCost}{$LOCperModule.v2$} $* cacheBreaks$
		\State $costChange += cost$
	\EndFor 
	\For{$(v1,v2) \in TDr$}
		\State $cacheBreaks \gets ROCpM.v2 - ModsCT.v1.v2$
		\State $cost \gets $\Call{LOCtoCost}{$LOCperModule.v2$} $* cacheBreaks$
		\State $costChange -= cost$
	\EndFor 

	\Return $costChange$
\EndFunction

\end{algorithmic}
\end{algorithm}
